# Supplementary material for: Experimental observation of polarization-dependent ultrafast carrier dynamics in multi-layer graphene
Source: arXiv:1301.1743 source file (2013-02-28)
Supplement: Supplementary file 1 [file Supplemental_Material_Yan_et_al.pdf]

## Experimental observation of polarization-dependent ultrafast carrier dynamics in multi-layer graphene

Xiao-Qing Yan<sup>1,2</sup>, Zhi-Bo Liu<sup>1,\*</sup>, Jun Yao<sup>1</sup>, Xin Zhao<sup>1</sup>, Xu-Dong Chen<sup>1</sup>, Xiang-Tian Kong<sup>1</sup>,  
Fei Xing<sup>1</sup>, Yongsheng Chen<sup>2</sup>, Jian-Guo Tian<sup>1,\*</sup>

<sup>1</sup>The Key Laboratory of Weak Light Nonlinear Photonics, Ministry of Education, Teda Applied Physics School, and School of Physics, Nankai University, Tianjin 300457, China

<sup>2</sup>The Key Laboratory of Functional Polymer Materials and Center for Nanoscale Science & Technology, Institute of Polymer Chemistry, College of Chemistry, Nankai University, Tianjin 300071, China

### 1. Reflectance and transmittance of probe beam when the pump beam was blocked

The dependence of reflected/transmitted probe beam signal from the two setups (Fig. 1 in main text) on polarization of probe beam was measured when the pump beam was blocked (Fig. S1). For the case of total internal reflection (TIR) (Fig. S1a), the reflectance is lowest for *s*-polarized light and largest for *p*-polarized light. However, for the case of non-total internal reflection (nTIR), the reflectance is largest for *s*-polarized light and lowest for *p*-polarized light as shown in Fig. S1b. Conversely, the transmittance is largest for *p*-polarized light and smallest for *s*-polarized light under the case of non-total internal reflection (Fig. S1c). For TIR, there is no transmittance from the oblique face of right-angle prism for probe beam. The polarization dependences of reflectance and transmittance could be well fit with the theory in [1,2], as the solid black lines shown in Fig. S1. The theoretical analysis was based on the boundary continuity of Maxwell' equitation. For TIR, the polarization dependence is mainly caused by difference of electric energy density for *s*- and *p*-polarized beam [1,2].

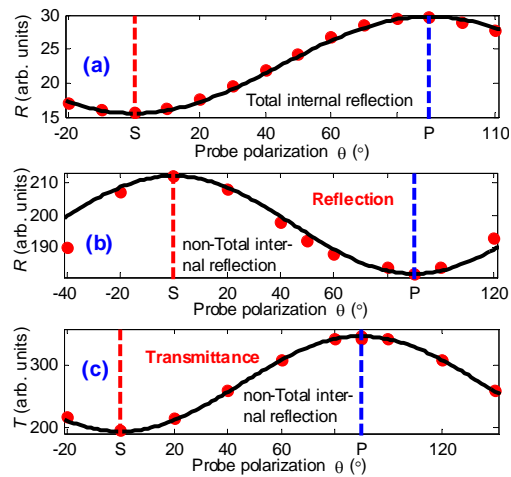

Fig. S1. Polarization dependence of linear reflectance of probe beam for the cases of total internal reflection (a) and non-total internal reflection (b). Linear transmittance of probe beam as function of probe polarization for the case of non-total internal reflection (c). The solid black lines are from theoretical fittings.

## A. Total internal reflection case

### 2. Differential reflectivity $\Delta R/R$ measurements for different polarized probe beam under the excitation of $p$ -polarized pump beam for TIR

Experimental results in Fig. S2 show differential reflectivity  $\Delta R/R$  measurements for different polarized probe beam under  $p$ -polarized pump beam excitation. The peak differential reflectivity  $\Delta R/R$  signal around 0 ps delay is largest for  $p$ -polarized probe beam and smallest for  $s$ -polarized. The probe polarization dependence of  $\Delta R/R$  signal during pulse excitation is opposite to that under  $s$ -polarized pump beam excitation (Fig. 2a in main text). The maximum differential reflectivity  $\Delta R/R$  around 0 ps delay time could be obtained by using probe beam with the same polarization as pump beam.

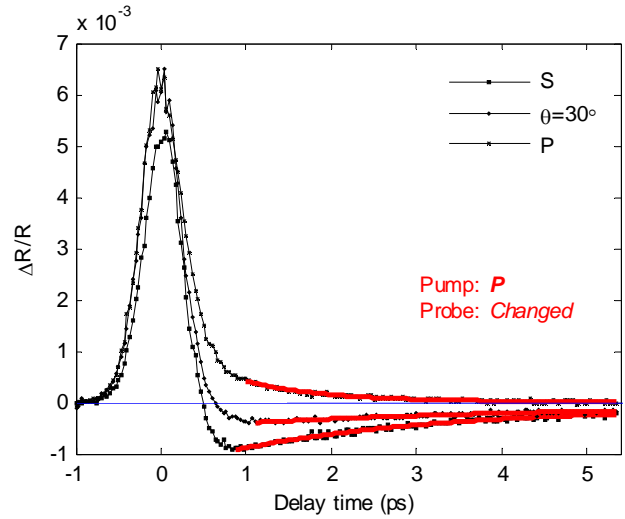

Fig. S2. The degenerate differential reflectivity  $\Delta R/R$  for probe beam with different polarization under the excitation of  $p$ -polarized pump beam.

### 3. Pump fluence dependence of maximum and minimum differential reflectivity $\Delta R/R$

Figures S3a-d show a linear power dependence of transient signals for different polarization combination of pump and probe beams, which means the signal is from single photon process [4-5]. The minimum  $\Delta R/R$  signal at valley of  $\Delta R/R$  curves of  $s$ -polarized probe beam is shown in Figs. 5e and f for  $s$ - and  $p$ -polarized pump beam, respectively. The minimum  $\Delta R/R$  signal enhances with pump fluence at low pump fluence, at high pump fluence this value does not change with fluence. An opposite

pump fluence dependence of the minimum negative differential transmittance signal ( $\min(\Delta T/T)$ ) was reported in [6]. In their measurements, the differential transmittance signal was measured with beams normal incident into graphene and the probe and pump beams are collinearly polarized [6,7].

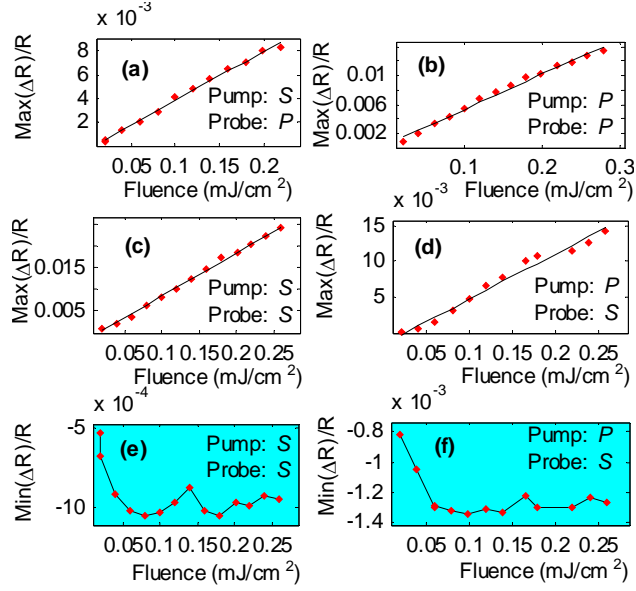

Fig. S3. Linear dependence of the maximum differential reflectivity  $\Delta R/R$  on pump fluence for different pump-probe combination, the linear fit is denoted by the solid line (a,b,c,d). The dependence of minimum differential reflectivity  $\Delta R/R$  value around 1 ps delay time on pump fluence (e,f).

## B. non-Total internal reflection case: Reflectance

### 4. Probe polarization dependent differential reflectivity $\Delta R/R$ measurements for nTIR

Figure S4 presents transient differential reflectivity  $\Delta R/R$  signal for different polarized probe beam when the pump polarization is  $\theta=130^\circ$ . The transient differential reflectivity  $\Delta R/R$  curves for probe beam with  $\theta=66\sim 72^\circ$  are shown in Fig. S4b. From the figures, we find that the  $\Delta R/R$  signal around 0 delay time is positive for *s*-polarized probe beam, and the signal could be continuously altered to negative.

From Fig. S4a and the continuously changing tendency for  $\Delta R/R$  signal at 0 delay time, we prone to believe there is one polarization for probe beam without  $\Delta R/R$  signal from absorption change. But, we still observed tiny non-absorption change signal in the transient differential reflectivity  $\Delta R/R$  curve in Fig. S4b. Part of the observed signal may from two-beam coupling effect caused by stimulated Rayleigh-wing scattering [8-9]. So, there was possible nuclear nonlinearity contribution in the measurements for the femtosecond laser pulses used here [10], and the two-beam coupling signal was much smaller than the signal from absorption change for *s*- or *p*-polarized probe beam. Indeed, there is no signal in the differential

reflectivity  $\Delta R/R$  curve for probe polarization of  $\theta=68^\circ$  when the pump polarization is  $\theta=40^\circ$  (Fig. 3a of main text).

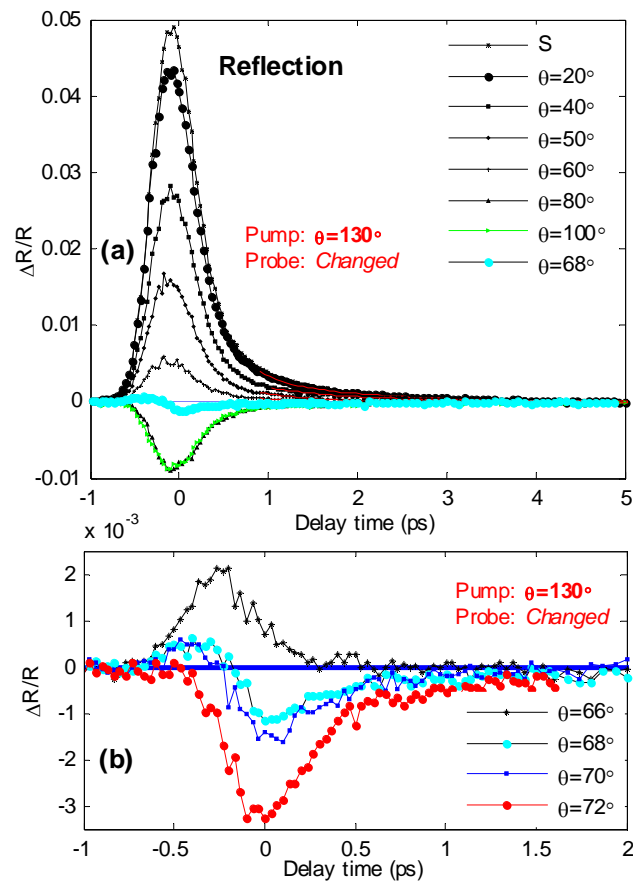

Fig. S4. (a) The degenerate differential reflectivity  $\Delta R/R$  for different polarized probe beam under the pump fluence of  $0.2 \text{ mJ/cm}^2$  and pump polarization  $\theta=130^\circ$ . (b) The degenerate differential reflectivity  $\Delta R/R$  for different polarized probe beam.

## 5. Pump fluence dependence of maximum/minimum values of differential reflectivity $\Delta R/R$ around 0 ps delay time

The peak/valley value of differential reflectivity  $\Delta R/R$  around 0 ps delay time changes linearly with pump fluence for *s*-/*p*- polarized probe beam as shown in Fig. S5. It means that the differential reflectivity  $\Delta R/R$  signal is from single photon absorption blocking process no matter what the polarizations of beams are [4,5].

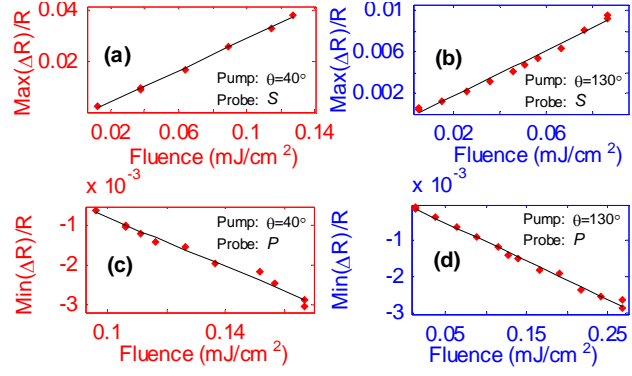

Fig. S5. Linear dependence of maximum/minimum differential reflectivity  $\Delta R/R$  value around 0 ps delay time on pump fluence for different pump-probe polarization combination, solid lines are from linear fits.

## C. non-Total internal reflection case: Transmittance

### 6. Polarization dependence of maximum differential transmittance $\Delta T/T$ around 0 ps delay time for nTIR

Figures S6a-b show the probe polarization dependence of maximum transmittance change  $\Delta T/T$  under *p*-/*s*- polarized pump beam excitation. No matter what the pump polarization is, the maximum differential reflectivity  $\Delta T/T$  is largest for *s*-polarized probe beam and decreases monotonously when the probe polarization was altered from S to P.

Figures S6c-d show the pump polarization dependence of maximum transmittance  $\Delta T/T$  change for *p*- and *s*-polarized probe beam, respectively. As the case of reflectance, the differential transmittance  $\Delta T/T$  is maximum when the pump polarization is identical to probe polarization.

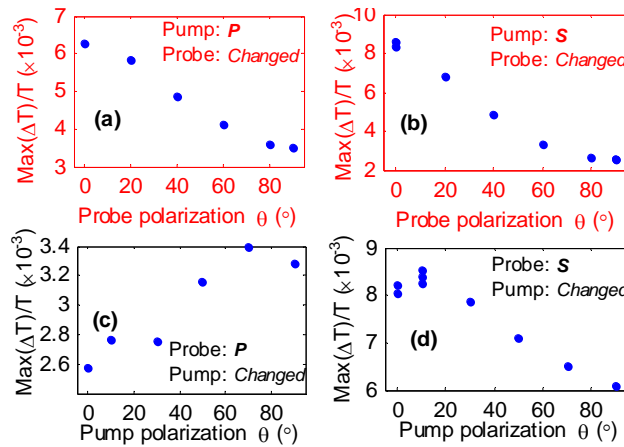

Fig. S6. The peak differential transmittance  $\Delta T/T$  around 0 ps delay time as function of the probe/pump polarization with pump/probe polarization fixed.

## 7. Pump fluence dependence of peak values of differential transmittance $\Delta T/T$ around 0 ps delay time

As the reflectance case, the maximum differential transmittance  $\Delta T/T$  depends linearly on pump fluence for different pump-probe polarization combination.

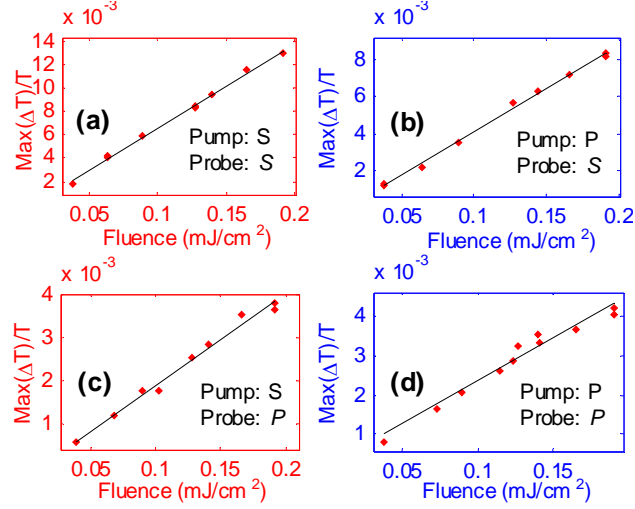

Fig. S7. Linear pump fluence dependence of the peak differential transmittance  $\Delta T/T$  around 0 ps delay time for different pump-probe polarization combination, solid lines are from linear fits.

## References

1. Q. Ye, J. Wang, Z.-B. Liu, Z.-C. Deng, X.-T. Kong, F. Xing, X.-D. Chen, W.-Y. Zhou, C.-P. Zhang, J.-G. Tian, Appl. Phys. Lett. 102, 021912 (2013).
2. F. Xing, Z.-B. Liu, Z.-C. Deng, X.-T. Kong, X.-Q. Yan, X.-D. Chen, Q. Ye, C.-P. Zhang, Y.-S. Chen & J.-G. Tian, Scientific Reports 2, 908 (2012).
3. K. Seibert, G. C. Cho, W. Kutt, H. Kurz, D. H. Reitze, J. I. Dadap, H. Ahn, and M. C. Downer, A. M. Malvezzi, Phys. Rev. B 42(5), 2842 (1990).
4. M. Breusing, S. Kuehn, T. Winzer, E. Milde, N. Severin, J.P. Rabe, C. Ropers, A. Knorr, and T. Elsaesser, Phys. Rev. B 83, 153410 (2011).
5. M. Breusing, C. Ropers, and T. Elsaesser, Phys. Rev. Lett. 102, 086809 (2009).
6. Dong Sun's dissertation, *Hot dirac fermion dynamics and coherently controlled photocurrent generation in epitaxial graphene*.
7. D. Sun, Z.-K. Wu, C. Divin, X. Li, C. Berger, W. A. de Heer, P. N. First, and Theodore B. Norris, Phys. Rev. Lett. 101, 157402 (2008).
8. A. Dogariu, T. Xia, D. J. Hagan, A. A. Said, E. W. Van Stryland, and N. Bloembergen, J. Opt. Soc. Am. B 14, 796-803 (1997).
9. C. Li, K. Yang, Y. Feng, X. Su, J. Yang, X. Jin, M. Shui, Y. Wang, X. Zhang, Y. Song and H. Xu, J. Phys. Chem. B, 113 (48), 15730-15733 (2009).
10. R. W. Boyd, *Nonlinear Optics*, 2nd ed. (Academic Press, San Diego, 2003).
